# Supplementary material for: Signatures of magnetic-field-driven quantum phase transitions in the entanglement entropy and spin dynamics of the Kitaev honeycomb model
Source: arXiv:1805.03722 source file (2019-04-30)
Supplement: Supplementary file 1 [file Supplemental_1805.03722.pdf]

# Supplementary Material for
# "Signatures of magnetic field driven quantum phase transitions in the entanglement entropy and spin dynamics of the applied field Kitaev honeycomb model"


David C. Ronquillo, Adu Vengal, and Nandini Trivedi

*Department of Physics, The Ohio State University, Columbus, Ohio 43210, USA*



(Dated: April 29, 2019)


## 16 AND 24 SITE CLUSTERS WITH PERIODIC BOUNDARY CONDITIONS

In calculating the energy spectrum and the topological entanglement entropy (using exact diagonalization (ED)) presented in Fig. 1 of the main text we employed the 24 site parallelogram shaped cluster shown on the right hand side of Fig. 1 below. The spin dynamics results presented in the main text were obtained employing the 16 site rectangular shaped cluster shown on the left hand side of Fig. 1 below. For each of these, we employed periodic boundary conditions.

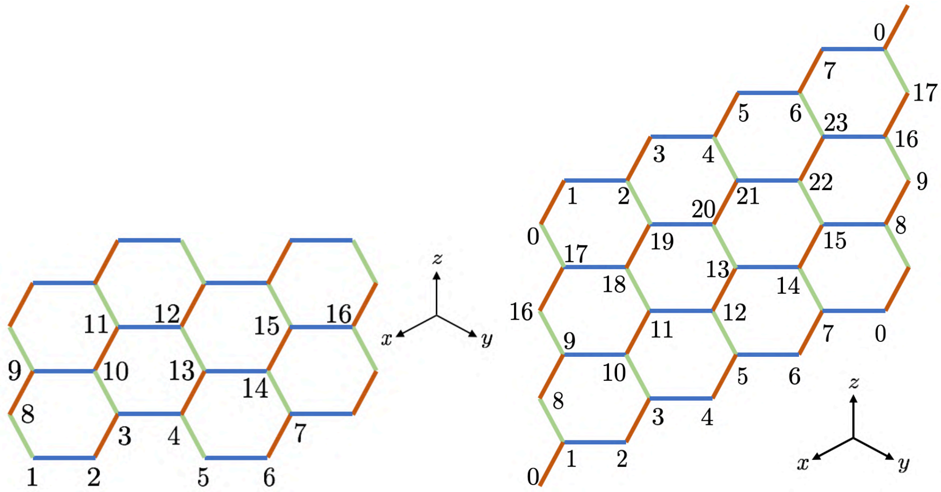

FIG. 1: 16 (left) and 24 (right) site clusters consisting of eight and 12 plaquettes, respectively. We used periodic boundary conditions in our ED simulations. Blue bonds correspond to $z-$bonds, green bonds correspond to $x-$bonds, and red bonds correspond to $y-$bonds.

## TIME-DEPENDENT SPIN-SPIN CORRELATION FUNCTIONS

As we reference in the main text, below we show $S^{zz}_{1,1}(\omega, \theta = \text{constant})$ cuts along the following constant values of the magnetic field strength parameter $\theta = \tan^{-1}(|\vec{h}|/J) \simeq 0, 0.28, 0.50, 1.01$, and 1.57, corresponding to the horizontal green dashed lines in Fig. 2a of the main text, for a field pointing along the [111] direction. For $\theta = 0$ (Fig. 2a below) we clearly see the dominant lower energy flux-gap mode, along with the higher energy less intense modes that are responsible for yielding the waveform shown Fig. 3a of the main text. Figure 2b below, corresponding to a cut just below the phase transition line between the gapped Kitaev QSL and the new gapless intermediate QSL ($\theta \approx 0.28$, see Fig. 2 of the main text), shows the drastic decrease in the intensity of the formerly most prominent modes in the $\theta = 0$ case in Fig. 2a below. Increasing the field strength until we are well within the gapless intermediate regime ($\theta \approx 0.50$, Fig. 2c below) we see the diminishment of all formerly prominent modes (at lower field strengths) except for a single low energy mode near $\theta \approx 0.75$. The overall decrease in the intensity of modes across all $\omega$ is also reflected in the sum over intensities across all $\omega$ shown in Fig. 2b of the main text. At $\theta \approx 1.01$, Fig. 2d below reflects the increase in the intensity of modes, particularly towards lower $\omega$, with the majority of the intensity concentrated in two distinctly sharp modes. In the final panel (Fig. 2e below) we see the modes in panel Fig. 2d have evolved into a

single dominant mode at maximum polarization, $\theta = \pi/2$. We have checked that the eigenstate corresponding to this latter mode is that of a single spin flip, and is thus the excited magnon mode of a fully polarized system. Finally, a sharp mode with significant intensity is also seen at $\omega = 0$, for $\theta = \pi/2$.

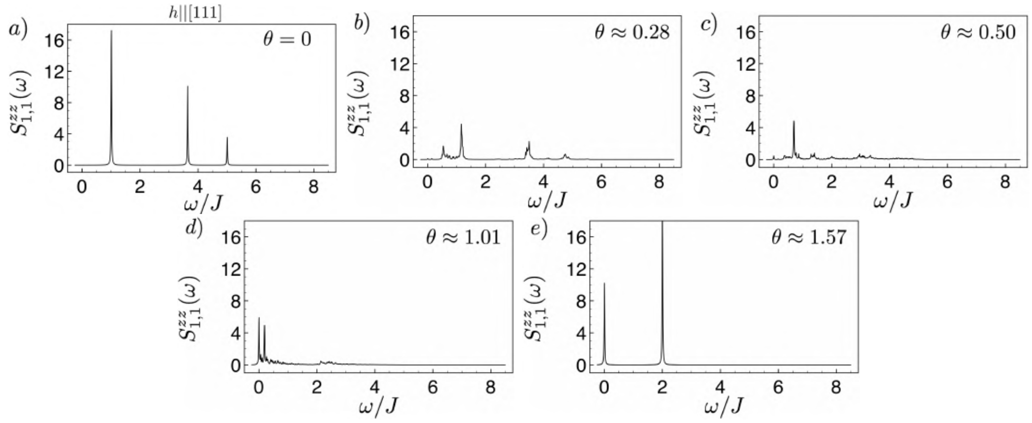


FIG. 2: Cuts along constant values the field strength parameter, $\theta$, of the local dynamical response (Fig. 2a in main text) for a field pointing along [111] (a-e).

## IMPORTANCE OF CLUSTER GEOMETRY TO CONSISTENCY IN NUMERICAL RESULTS

For equal sized clusters, the choice of cluster geometry used in performing one's finite size ED calculations will noticeably affect the quantitative results obtained. To demonstrate the extent of the expected numerical discrepancy that may be attributed to the different choice of cluster geometry, we highlight the 24 site zero-field ED low lying spectrum results obtained in Ref. [1], wherein a C3 symmetric cluster (left hand side of Fig. 3 below) was employed: $E_1 \approx 0.034$, $E_2 \approx 0.051$, $E_3 \approx 0.088$, $E_4 \approx 0.094$ (where $E_1$, $E_2$, $E_3$, and $E_4$ are the lowest lying excited eigenenergies) and compare these with the 24 site zero-field ED low lying spectrum results obtained in Ref. [2], wherein a parallelogram shaped cluster (right hand side of Fig. 3 below) was instead employed: $E_1 \approx 0.026$, $E_2 \approx 0.067$, $E_3 \approx 0.075$, $E_4 \approx 0.078$.

For the results presented in our main text, we employed a 24 site parallelogram shaped cluster, like the one employed in [2]. This explains the complete agreement we share in our zero-field ED low lying spectrum results (Fig. 1 of our main text) with the results found in Ref. [2] (and not with those found in Ref. [1]), after accounting for a missing 1/4 factor deriving from the fact that we employed Pauli operators ($\sigma^\alpha$, with $\alpha = x, y, z$) instead of spin operators ($S^\alpha$) in carrying out our numerics (our corresponding zero-field data: $E_1 \approx 0.105 \times (1/4) \approx 0.026$, $E_2 \approx 0.27 \times (1/4) \approx 0.067$, $E_3 \approx 0.301 \times (1/4) \approx 0.075$, $E_4 \approx 0.314 \times (1/4) \approx 0.078$).

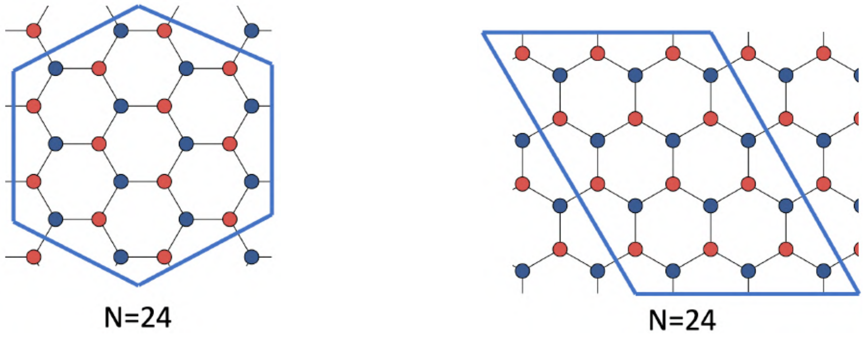


FIG. 3: 16 (left) and 24 (right) site clusters consisting of eight and 12 plaquettes, respectively. We used periodic boundary conditions in our exact diagonalization simulations. Blue bonds correspond to $z-$bonds, green bonds correspond to $x-$bonds, and red bonds correspond to $y-$bonds.

Finally, we demonstrate the correspondence between the location of the phase transition between the non-Abelian gapped Kitaev phase and the intermediate gapless QSL phase, for a field pointing along [111], obtained by us (Fig. 1 of the main text) and by Ref. [2]. Each of us having, respectively, used the same 24 site parallelogram shaped cluster for our ED calculations, we assessed the location of the phase transition point by estimating the location of the level crossing point between the lowest lying excited state energy and the ground state energy (for Ref. [2] $H_{111} \approx 0.2$, versus our $\theta \approx 0.62$).

The Hamiltonian we employed for a field pointing along $\vec{h} = [111]$ is given by

$$H_{\mathrm{DR}} = J \sum_{\alpha} \sum_{\langle i,j \rangle} \sigma_i^{\alpha} \sigma_j^{\alpha} - h \sum_{i,\alpha} \frac{1}{\sqrt{3}} \sigma_i^{\alpha}, \tag{1}$$

which we now compare to the Hamiltonian employed by Ref. [2] for a field pointing along $\vec{h} = [111]$

$$\begin{aligned} H_{\mathrm{ZZ}} &= \sum_{\alpha} \sum_{\langle i,j \rangle} K\, S_i^{\alpha} S_j^{\alpha} - H_{111} \sum_{i,\alpha} S_i^{\alpha} & (2) \\ &= \sum_{\alpha} \sum_{\langle i,j \rangle} \frac{1}{4} K \sigma_i^{\alpha} \sigma_j^{\alpha} - \frac{\sqrt{3}}{2} H_{111} \sum_{i,\alpha} \frac{1}{\sqrt{3}} \sigma_i^{\alpha} & (3) \end{aligned}$$

Observe,

$$\begin{aligned} \left(\frac{h}{J}\right)_{\mathrm{DR}} &= \tan(\theta) = \tan(0.62) \approx 0.71 & (4) \\ &\approx \frac{\frac{\sqrt{3}}{2} H_{111}}{\frac{1}{4} K} = 2\sqrt{3} \left(\frac{H_{111}}{K}\right) = 2\sqrt{3}\,(0.2) \approx 0.69, & (5) \end{aligned}$$

for $J = K = 1$. Thus, our estimates for the location of the phase transition are consistent; unsurprisingly, since we each employed the same 24 site geometry in our ED calculations.

---

C. Hickey and S. Trebst, Nature Communications **10**, 530 (2019), ISSN 2041-1723, `https://doi.org/10.1038/s41467-019-08459-9`.

Z. Zhu, I. Kimchi, D. N. Sheng, and L. Fu, Phys. Rev. B **97**, 241110 (2018), `https://link.aps.org/doi/10.1103/PhysRevB.97.241110`.
